# Supplementary material for: Stirrers and movers actuated by oscillating fields
Source: arXiv:1607.04733 source file (2016-09-13)
Supplement: Supplementary file 1 [file supplementary.pdf]

# Supplementary Information:
# Stirrers and movers actuated by oscillating fields

Gabi Steinbach,[1,2] Michael Schreiber,[1] Dennis Nissen,[3] Manfred Albrecht,[3] Sibylle Gemming,[1,2] and Artur Erbe[2]

[1]*Institute of Physics, Technische Universität Chemnitz, D-09107 Chemnitz, Germany.*
[2]*Helmholtz-Zentrum Dresden-Rossendorf, Institute of Ion Beam Physics and Materials Research, Bautzner Landstrasse 400, 01328 Dresden, Germany.*
[3]*Institute of Physics, University of Augsburg, 86159 Augsburg, Germany.*

## ANALYTICAL CALCULATION OF THE SINGLE-PARTICLE DISPLACEMENT

A dipolar sphere that is exerted to a magnetic torque rotates around its magnetic center. If the magnetic center is shifted away from the geometric center, as given for sd-particles, then the rotation leads to a displacement of the sphere center. The path of motion is an arc (Fig. S1) with a radius determined by the magnetic shift, $\xi\frac{d_p}{2}$. Here, the displacement of an sd-particle that rotates in response to an external field pointing along the $z$-axis is considered. The displacement of sd-particles caused by the rotation by an angle $\theta$ in an isotropic medium can be expressed analytically. When rotating about the magnetic center (dipole position), the ideal displacements perpendicular ($r$) and parallel ($z$) to an oscillating field $B^z$ are given by

$$r = \xi(\cos\theta - 1)\frac{d_\mathrm{p}}{2}\ , \quad z = \xi\sin\theta\frac{d_\mathrm{p}}{2}. \qquad \text{(S1)}$$

In viscous medium, translational drag reduces this displacement, which can be considered as an reduced effective shift of the magnetic center. In an isotropic medium, viscous drag leads to a constant reduction factor. It has been disregarded here since for a qualitative description of the actuation concept only anisotropic drag is relevant. From the differentiation of $r$ and $z$ with respect to $\theta$ one obtains the infinitesimal displacements

$$\mathrm{d}r = \mathrm{d}\theta\, c(\theta)\,\xi(-\sin\theta)\frac{d_\mathrm{p}}{2}\ , \quad \mathrm{d}z = \mathrm{d}\theta\, c(\theta)\,\xi\cos\theta\frac{d_\mathrm{p}}{2}. \qquad \text{(S2)}$$

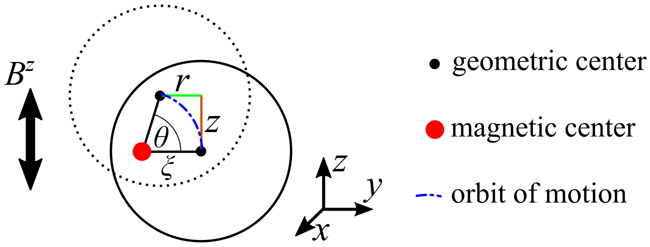


Fig. S 1. Sketch of a sphere before (solid circle) and after (dotted circle) rotation by $\theta$ around the magnetic center that is shifted by $\xi$. The center of the sphere moves by $r = \sqrt{x^2 + y^2}$ ($\perp B^z$) and $z$ ($\parallel B^z$).

An additional term $c(\theta)$ has been incorporated here. It accounts for sources of anisotropic friction that hinder or enhance this displacement.

## CALCULATION OF THE TRANSLATION IN A RING CLUSTER

The time-dependent translation $r(t)$ of sd-particles along the orbit of the triple ring can be calculated by integrating Eq. S2 after inserting analytic expressions for $\varphi(t)$, $\theta(t)$, and $c(\theta) = \cos(\varphi(\theta(t)))$. The expressions are obtained by fitting the steady-state trajectory $\varphi(\theta)$ (Fig. 3 b) to a Lissajous curve. The fitting curve has the form

$$\varphi(\theta) = \varphi_A \sin\left(2\arcsin\frac{\pm\theta}{\theta_A} + p\right) + n \qquad \text{(S3)}$$

with the azimuthal and the radial amplitudes $\varphi_A$ and $\theta_A$, the phase shift $p$ between $\varphi$ and $\theta$ and the offset $n$ of the angle $\varphi$ caused by the dipole shift. The sign $\pm$ accounts for the fact that $\varphi(\theta)$ is a multivalued function. $\varphi$ and $\theta$ perform harmonic oscillations with a frequency ratio of $\omega_\varphi/\omega_\theta = 2$. $\omega_\theta$ equals the frequency of the external, oscillating field, $\omega_\mathrm{B}$. With the fit parameters $\varphi_A, \theta_A, p, n$, the time-dependent torsional oscillations of the particles in a ring can be expressed by $\varphi(t) = \varphi_A \sin(2\omega_\mathrm{B}t + p) + n$ and $\theta(t) = \theta_A \sin(\omega_\mathrm{B}t)$. From the differentiation $\frac{\mathrm{d}\theta(t)}{\mathrm{d}t}$ we obtain the substitution for the integration variable as $\mathrm{d}\theta = \mathrm{d}t\,\theta_A\omega_\mathrm{B}\cos(\omega_\mathrm{B}t)$. After inserting these expressions into Eq. S2, the time-dependent translation is obtained from the integration $r(t') = \int_0^{t'} \mathrm{d}r(t)$. For particles in a ring that is located on a surface, it has to be taken into account that $c(\theta) = \cos\varphi(\theta(t)) \cdot c_\mathrm{f}(\theta)$.

## SHAPE AND MASS ANISOTROPY OF CAPPED PARTICLES

The hemispherical coating of the studied silica spheres theoretically leads to shape anisotropy and mass imbalance. Here, we have deposited a metallic film with a maximum thickness of $t_0 = 16.5\,\mathrm{nm}$ onto an array of silica spheres with a diameter of $d_\mathrm{p} = 4.5\,\mu\mathrm{m}$. Deposition normal to the array leads to a hemispherical coverage of

each particle. Across the coated hemisphere, the thickness $t$ of the film varies as $t_0 \cos\alpha$ with the polar angle $\alpha$ measured with respect to the symmetry axis (Janus director). The film deposition leads to a maximum variation of the particle diameter of $t_0/d_\mathrm{p} = 0.0036$, which is negligibly small. This justifies our assumption that capped particles are still spherical.

To calculate the center of mass of the coated particles, additionally, the different mass densities $\rho$ of the spheres and of the metal film have to be regarded. The silica spheres have a density of $\rho_\mathrm{Si} = 2\frac{\mathrm{g}}{\mathrm{cm}^3}$. For the metal film, we estimate a mean density of $\rho_\mathrm{F} = 12.4\frac{\mathrm{g}}{\mathrm{cm}^3}$, which follows from the densities of each element in the film (Ta: $16.6\frac{\mathrm{g}}{\mathrm{cm}^3}$; Co: $8.9\frac{\mathrm{g}}{\mathrm{cm}^3}$; Pd: $12.0\frac{\mathrm{g}}{\mathrm{cm}^3}$) and their relative fraction of the total film thickness (Ta: 18 % ; Co: 13 % ; Pd: 69 % ). Due to the rotational symmetry of the coated particle, the center of mass is located on the symmetry axis. In the following, this axis is defined as $z$, and the center of the silica sphere is located at $z = 0$. The center of mass, $z_\mathrm{m}$ is given by

$$z_\mathrm{m} = \frac{\int \mathrm{d}V\, z\rho}{\int \mathrm{d}V\, \rho} \tag{S4}$$

The numerator of this fraction reduces to the cap since the integration $\int \mathrm{d}V\, z\rho$ over the silica sphere is zero. For the cap, we transform into spherical coordinates with polar angle $\alpha$ and azimuth angle $\beta$, and we can substitute $z = \frac{d_\mathrm{p}}{2}\cos\alpha$. For the hemispherical cap ($\alpha \in [-\frac{\pi}{2} : \frac{\pi}{2}]$, $\beta \in [0 : 2\pi]$) with film thickness $t_0 \cos\alpha$, this gives

$$\int_\mathrm{cap} \mathrm{d}V\, z\rho = \int_0^{2\pi} \mathrm{d}\beta \int_{-\frac{\pi}{2}}^{\frac{\pi}{2}} \mathrm{d}\alpha\, \frac{d_\mathrm{p}}{2}\cos\alpha\, \rho_\mathrm{F}\, t_0 \cos\alpha, \tag{S5}$$

which is $\pi^2 \frac{d_\mathrm{p}}{2}\, \rho_\mathrm{F}\, t_0$. The denominator of Eq. S4 is the total mass of the capped particle, consisting of a silica sphere and the cap of the metal film. This can be calculated by

$$\int_\mathrm{cap} \mathrm{d}V\, \rho = \frac{1}{6}\pi d_\mathrm{p}^3\, \rho_\mathrm{si} + \int_0^{2\pi} \mathrm{d}\beta \int_{-\frac{\pi}{2}}^{\frac{\pi}{2}} \mathrm{d}\alpha\, \rho_\mathrm{F}\, t_0 \cos\alpha, \tag{S6}$$

which gives $\frac{1}{6}\pi d_\mathrm{p}^3\, \rho_\mathrm{Si} + 4\pi\rho_\mathrm{F} t_0$. Inserting the solutions of Eq. S5 and Eq. S6 into Eq. S4 and taking the experimental values for the mass densities and the film thickness gives the mass center at $z_\mathrm{m} = 5 \cdot 10^{-5}$ nm. This corresponds to $10^{-6}$ % of $d_\mathrm{p}$, and, thus, the mass imbalance can be neglected here.

## MAGNETIC CONFIGURATIONS IN COMPACT CLUSTERS OF FIVE PARTICLES

The magnetic shift in anisotropic particles causes additional anisotropy of the magnetostatic potential between dipolar particles since the dipole interaction exhibits a distance dependence that is proportional to $1/r^3$. As a consequence of this anisotropy, particle assemblies exhibit magnetic configurations of the dipole orientations that strongly differ from those of typical dipolar particles. The capped particles can self-assemble in compact clusters, which can be reproduced with the model of sd-particles. Compact clusters of sd-particles exhibit a large variety of possible magnetic configurations [48]. In this work, clusters of three and five particles have been discussed. The configuration of a compact three particle cluster is unique. A ring forms and the caps (or dipoles) form a closed loop (Fig. 3 a, Fig. 4 a). For five particles, there also exists only one structural possibility for compact packing. However, the dipoles in this cluster can take different magnetic configurations. These configurations can be calculated numerically using sd-particles and conducting an energy minimization with respect to the dipole interaction. The same code as for the dynamic investigations has been employed here, but with the external field switched off. We have found seven different magnetic configurations (Fig. S2), which also differ in the magnetostatic energy. Two of them (Fig. S2 b and d) represent the two clusters of capped particles for which we have presented actuation here.

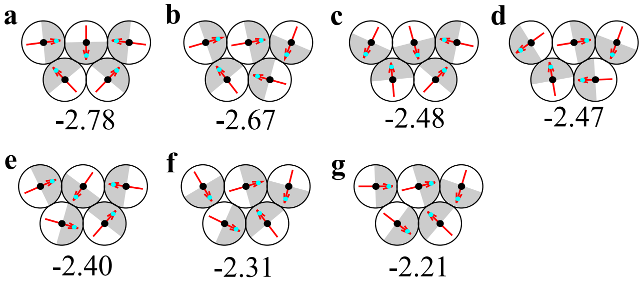


Fig. S 2. Clusters of five sd-particles ($\xi = 0.6$) with different magnetic configurations. There is only one possible structural configuration for a compact packing of five particles, but seven different magnetic configurations exist. Red arrows indicate the dipole orientations, and blue dots indicate the dipole positions. The hemisphere with the embedded dipole has been filled in grey to facilitate visual comparison with the experimental clusters. The numbers below the clusters give the magnetostatic energy per particle, measured in $\frac{\mu_0 m^2}{4\pi d_\mathrm{p}^3}$.
